# Supplementary material for: Multihyperuniform Long-Range Order in Medium-Entropy Alloys
Source: arXiv:2111.11412 source file (2021-11-22)
Supplement: Supplementary file 1 [file si_alloy_prl.pdf]

# Supplemental Materials: Multihyperuniform Long-Range Order in Medium-Entropy Alloys

Duyu Chen,[1,*] Xinyu Jiang,[2] Duo Wang,[2] Houlong Zhuang,[2,†] and Yang Jiao[3,4,‡]

[1]*Materials Research Laboratory, University of California, Santa Barbara, California 93106, United States*
[2]*Mechanical and Aerospace Engineering, Arizona State University, Tempe, AZ 85287*
[3]*Materials Science and Engineering, Arizona State University, Tempe, AZ 85287*
[4]*Department of Physics, Arizona State University, Tempe, AZ 85287*

## S1. NUMERICAL DETAILS FOR FOURIER-SPACE OPTIMIZATION TECHNIQUE

In this section, we provide details for our implementation of the Fourier-space optimization technique that we have developed to generate multihyperuniform and SQS alloys. Specifically, we start with random structures with prescribed concentrations/atomic fractions of different elements. At each time step we randomly select two atoms of different types, swap their positions, and accept the trial atom swap according to the probability

$$p_{acc}(old \to new) = \min\{1, \exp(-\frac{E_{new} - E_{old}}{T})\}, \tag{1}$$

where $T$ is the fictitious "temperature" of the system that is set initially high and gradually decreases according to a cooling schedule [1, 2], and $E_{new}$ and $E_{old}$ are the fictitious "energy" associated with the configuration after and before the particle swap, respectively. In particular, we typically start at an initial temperature $T_0$ such that the probability of accepting a particle swap move is around 50% and reduce the fictitious "temperature" of the system by a factor of $\alpha = 0.99$ after $n_{MC} = 1000$ particle swap moves, i.e., $T_{t+1} = \alpha T_t$, where $T_{t+1}$ and $T_t$ are the temperatures at temperature stage $t+1$ and $t$, respectively. We repeat the particle swaps until the "energy" $E$ essentially does not change. If the final $E$ is sufficiently close to zero, basically we have realized the system of interest with the targeted structure factors. Empirically, we find that 5000 and 600 temperature stages are generally sufficient for the generation of a multihyperuniform structure and a quasirandom structure with $N = 5832$ particles, respectively.

For computational purposes, the static structure factor $S(k)$ is the angular-averaged version of $S(\mathbf{k})$, which can be obtained directly from the particle positions $\mathbf{r}_j$, i.e.,

$$S(\mathbf{k}) = \frac{1}{N}\left|\mathcal{J}(\mathbf{k})\right|^2 \quad (\mathbf{k} \neq \mathbf{0}), \tag{2}$$

where the collection coordinate $\mathcal{J}(\mathbf{k})$ is defined as

$$\mathcal{J}(\mathbf{k}) = \sum_{j=1}^{N} \exp(i\mathbf{k}\cdot\mathbf{r}_j). \tag{3}$$

Note that the trivial forward scattering contribution ($\mathbf{k} = 0$) in Eq. 2 is omitted. To avoid the computation of $S(\mathbf{k})$ from scratch after each particle swap and greatly accelerate the computation, we keep track of $\mathcal{J}(\mathbf{k})$ for every individual element type in the alloy and update it according to

$$\mathcal{J}_{new}(\mathbf{k}) = \mathcal{J}_{old}(\mathbf{k}) + \exp(i\mathbf{k}\cdot\mathbf{r}_{new}) - \exp(i\mathbf{k}\cdot\mathbf{r}_{old}), \tag{4}$$

where $\mathbf{r}_{new}$ and $\mathbf{r}_{old}$ are the new and old particle positions after the particle swap for a given element type, respectively.

As a demonstration of the effectiveness and efficiency of our Fourier-space optimization scheme, we generate a single configuration of SQS with $N = 5832$ particles, which is supposed to reproduce the ensemble statistics of random mixtures. Indeed, as shown in Fig. S1, the structure factors $S(k)$ associated with the three individual elements in the generated SQS match extremely well with the targeted ensemble average of random mixtures, which is given by Eq. 3 in the main text. The generation of such a SQS generally takes less than a day on a single Intel(R) Core(TM) i7-6600U CPU (@ 2.60GHz).

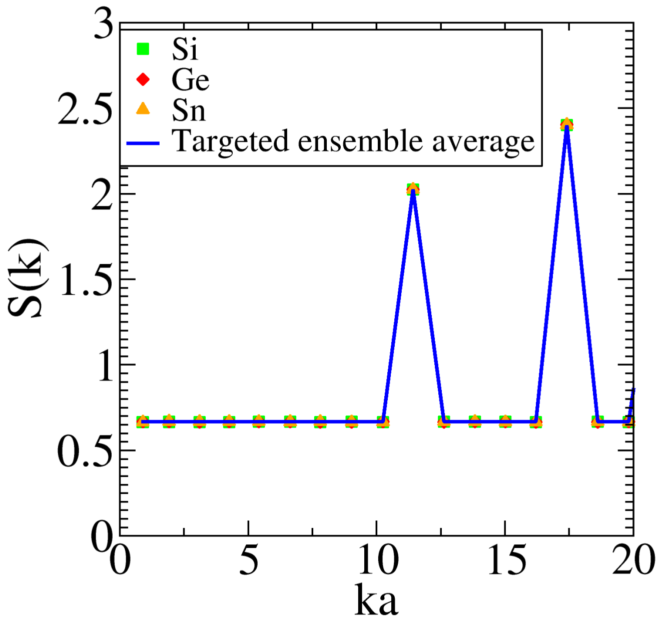


FIG. 1: Structure factors $S(k)$ of Si atoms, Ge atoms, and Sn atoms for a single realization of SQS, which match the corresponding ensemble average of random mixtures across length scales, consistent with the definition of SQS.

## S2. EFFECT OF EXCLUSION REGION ON THE STRUCTURAL CHARACTERISTICS OF MULTIHYPERUNIFORM ALLOYS

In this section we investigate the effect of exclusion region $K_0a$ on the generated multihyperuniform alloys. In particular, we suppress $S(k)$ over a larger range of $K_0a = 6$ compared to those configurations in the main text with $K_0a = 3.6$, and the statistics are shown in Fig. S2. Clearly, the structure factors $S(k)$ associated with the three elements in the *realized* multihyperuniform structures possess small, but finite values, and slowly increase as $k$ increases within the entire constrained region of $K_0a \leq 6$, and jump to much higher values once outside the constrained regions. Moreover, the repulsion of atoms of the same type from the neighboring shells of a given atom is much more significant in these configurations compared to those with a smaller exclusion region in the main text, indicating increased short-range chemical order as the exclusion region increases. This trend is expected due to the fact that as larger-wavenumber (or smaller-wavelength) correlations are constrained, clustering of atoms of the same type is further discouraged.

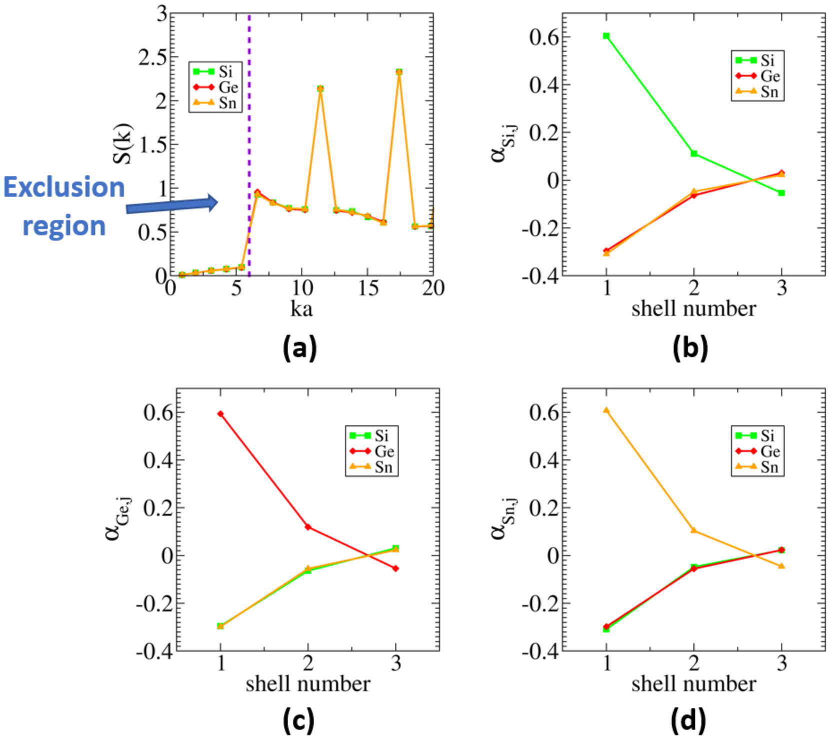


FIG. 2: Structure factors $S(k)$ associated with the three elements and short-range order parameters $\alpha_{ij}^{\nu}$ for multihyperuniform MEAs with an exclusion region of $K_0a = 6$. The results are averaged over 5 configurations with $N = 5832$ particles.

Next, we provide justification that the exclusion region $K_0a$ should be set sufficiently large in our optimization scheme to suppress the generation of periodic structures. In Fig. S2, we plot the structure factors associated with the three elements in a periodic structure with $N = 5832$ particles that is a periodic replica of a structure on a smaller $3 \times 3 \times 3$ diamond cubic lattice, as well as those in a disordered multihyperuniform structure at the same system size generated by our optimization scheme with an exclusion region of $K_0a = 3.6$. Clearly, the structure factors $S(k)$ for the periodic structure are absolutely zero at very small $k$ due to periodicity and thus stealthy by definition; however, when $K_0a$ is set to 3.6, the disordered multihyperuniform structure is still favored over the periodic structure in terms of its lower fictitious "energy" (defined in Eq. 1 in the main text), and indeed our optimization scheme is able to find such a disordered solution, which serves as the testament of the power of our algorithm. On the other hand, if $K_0a$ is further decreased beyond the wavenumber associated with the periodicity of the smallest repeating unit, the "energy" associated with the periodic structure will decrease to zero, and it will be favored over disordered structures. Therefore, it is important to set $K_0a$ sufficiently high so that we do not obtain a periodic structure, which is not a realistic structure for MEAs according to previous observations [3].

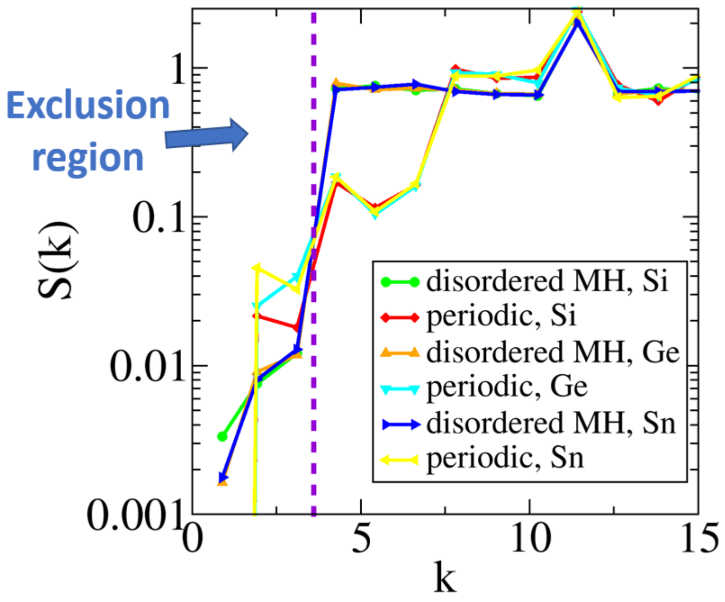


FIG. 3: Structure factors $S(k)$ associated with the three elements for a disordered multihyperuniform MEAs with an exclusion region of $K_0a = 3.6$ and $N = 5832$ particles compared to those of a periodic structure at the same system size that is a periodic replica of a structure on a smaller $3 \times 3 \times 3$ diamond cubic lattice with $N = 216$ particles.

## S3. ROBUSTNESS OF RESULTS TO SYSTEM SIZE

In this section we demonstrate that the salient structural features of our generated multihyperuniform MEAs are robust to the change of system size $N$. In particular, we generate such a configuration with $N = 46656$ particles on a $18 \times 18 \times 18$ diamond cubic lattice and with the same exclusion region of $K_0a = 3.6$ as those in the main text. We then compute the structures factors $S(k)$ associated with the three elements and short-range order parameters $\alpha^{\nu}_{ij}$, as shown in Fig. S4. The results at this system size $N = 46656$ are quantitatively similar to those of the corresponding systems at $N = 5832$ particles in the main text, indicating the robustness of the pair correlations and short-range orders of our generated multihyperuniform MEAs with respect to the system size.

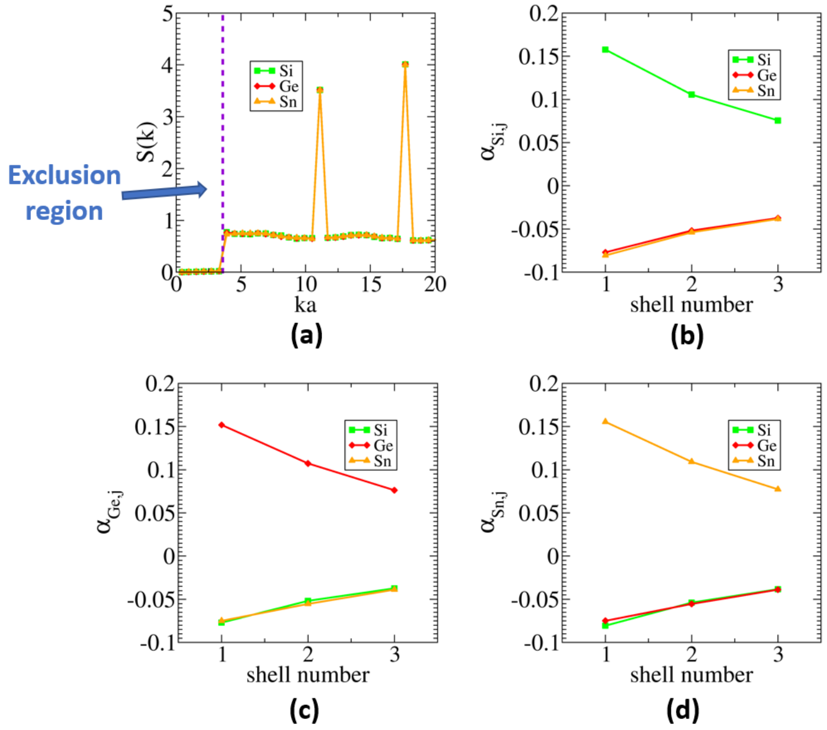


FIG. 4: Structure factors $S(k)$ associated with the three elements and short-range order parameters $\alpha_{ij}^{\nu}$ for multihyperuniform MEAs with an exclusion region of $K_0 a = 3.6$ and $N = 46656$ particles.

## S4. DENSITY FUNCTIONAL THEORY AND MOLECULAR DYNAMICS SIMULATION PARAMETERS

For a better comparison of multihyperuniform SiGeSn alloy to the corresponding alloy with a random structure, we use the same parameters as used in Ref. [4]. Here we provide a brief summary of these parameters. We use the Vienna Ab initio Simulation Package (VASP; version 5.4.4) [5] and the Perdew-Burke-Ernzerhof (PBE) functional [6] and projector augmented-wave (PAW) potentials [7, 8] for geometry optimizations and energy calculations and the modified Becke-Johnson (mBJ) exchange potential [9] for the band structures. The plane wave cutoff energy is 400 eV and a $2 \times 2 \times 2$ Monkhorst-Pack k-point grid [10] is used. All the DFT supercells have 216 atoms and the force convergence criterion is 0.01 eV/ Å. To obtain the thermal conductivity of the SiGeSn MEAs, we use the Large-scale Atomic/Molecular Massively Parallel Simulator (LAMMPS) [11] and a modified Stillinger-Weber potential [12–14].

* correspondence sent to: duyu@alumni.princeton.edu
† correspondence sent to: hzhuang7@asu.edu
‡ correspondence sent to: yang.jiao.2@asu.edu

[1] C. L. Y. Yeong and S. Torquato, Phys. Rev. E **57**, 495 (1998).
[2] C. L. Y. Yeong and S. Torquato, Phys. Rev. E **58**, 224 (1998).
[3] N. Muller, J. Haberko, C. Marichy, and F. Scheffold, Optica **4**, 361 (2017).
[4] D. Wang, L. Liu, M. Chen, and Z. H., Acta Mater. **199**, 443 (2020).
[5] G. Kresse and J. Furthmüller, Comput. Mater. Sci. **6**, 15 (1996).
[6] J. P. Perdew, K. Burke, and M. Ernzerhof, Phys. Rev. Lett. **77**, 3865 (1996).
[7] P. E. Blöchl, Phys. Rev. B **50**, 17953 (1994).
[8] G. Kresse and D. Joubert, Phys. Rev. B **59**, 1758 (1999).
[9] F. Tran and P. Blaha, Phys. Rev. Lett. **102**, 226401 (2009).

[10] H. J. Monkhorst and J. D. Pack, Phys. Rev. B **13**, 5188 (1976).
[11] S. Plimpton, J. Comput. Phys. **117**, 1 (1995).
[12] F. H. Stillinger and T. A. Weber, Phys. Rev. B **31**, 5262 (1985).
[13] Y. Lee and G. S. Hwang, Phys. Rev. B **85**, 125204 (2012).
[14] Y. Lee and G. S. Hwang, J. Phys. D: Appl. Phys. **50**, 494001 (2017).
